# Supplementary material for: Instant4D: 4D Gaussian Splatting in Minutes
Source: arXiv:2510.01119 source file (2025-10-01)

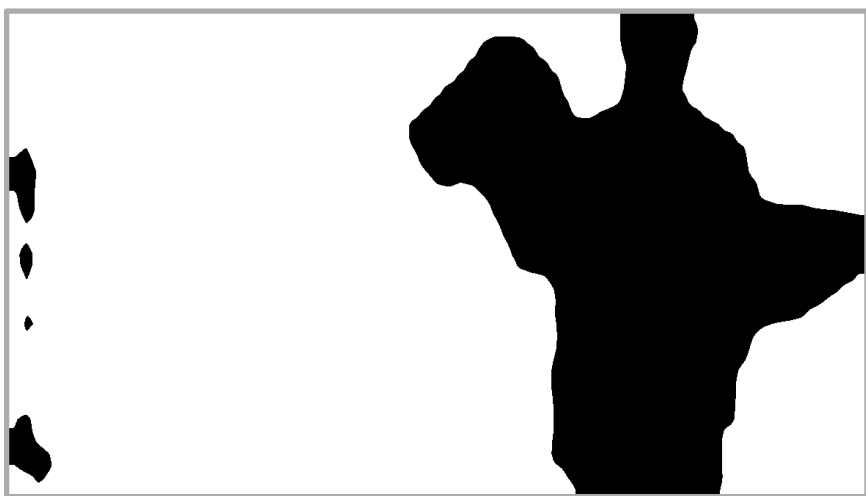

**Original**

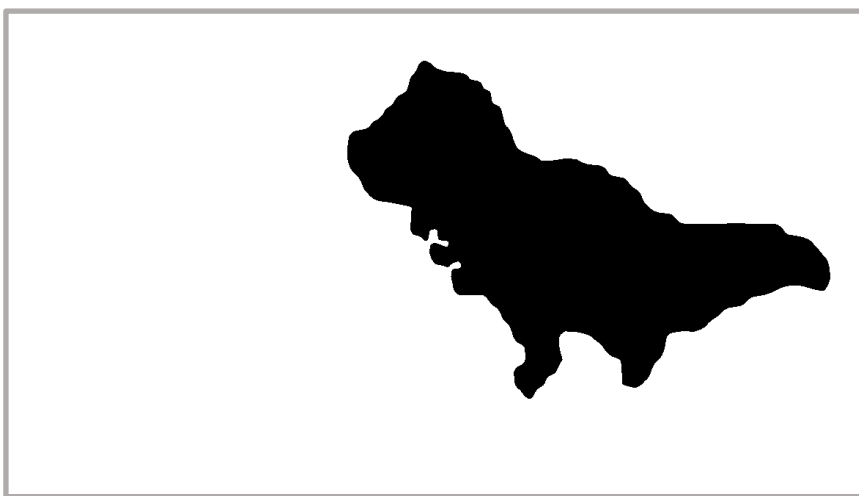

**Pseudo-frame**

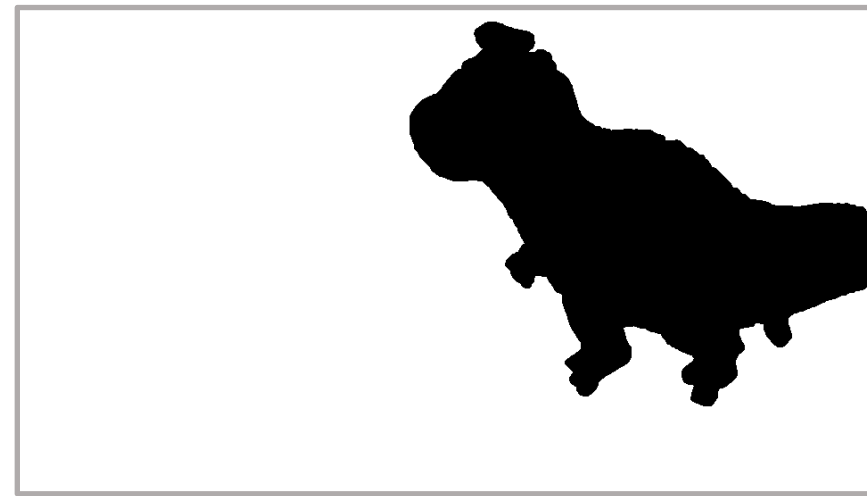

**Ground Truth Mask**

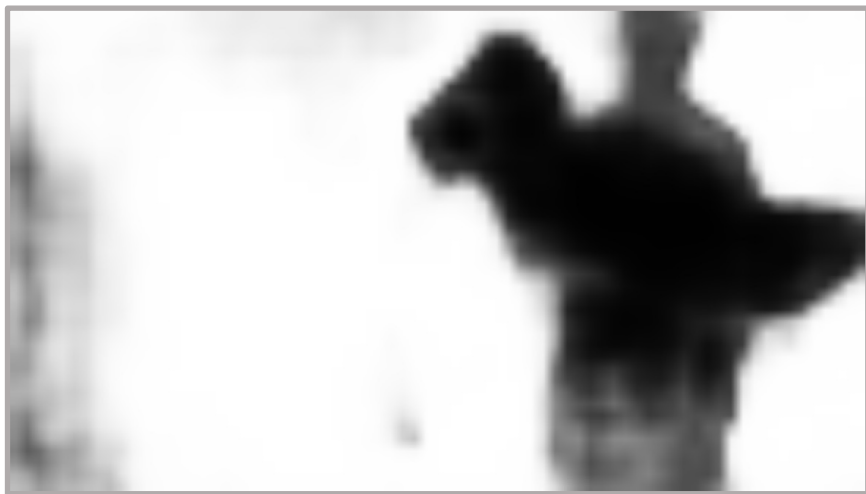

**Original**

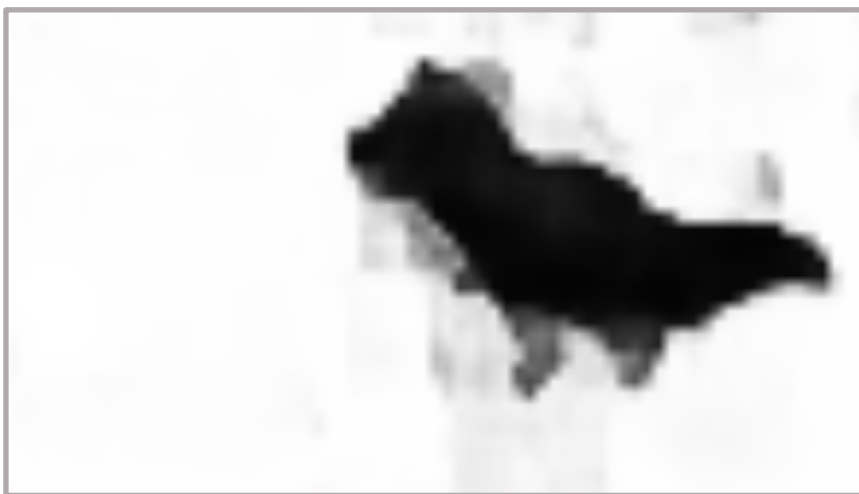

**Pseudo-frame**

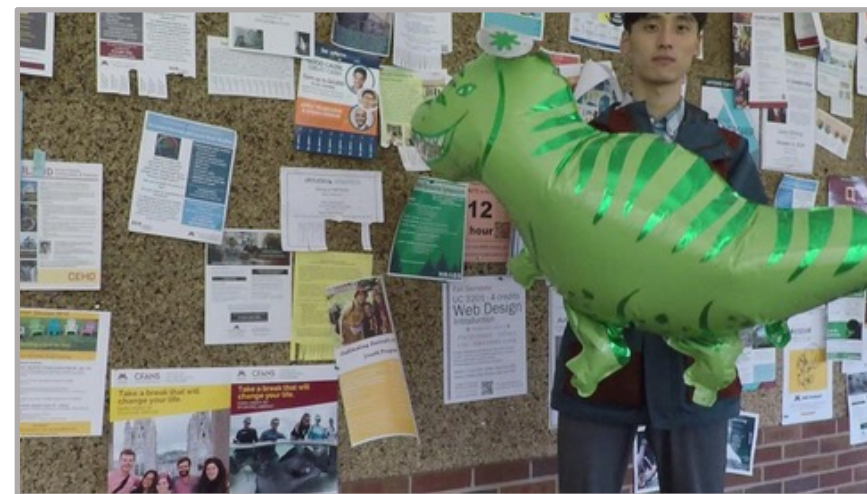

**Input Image**

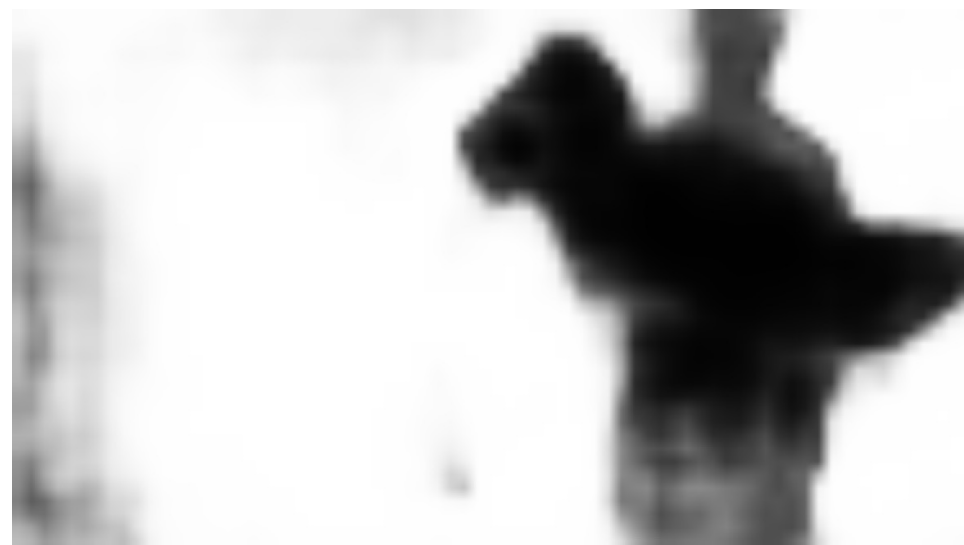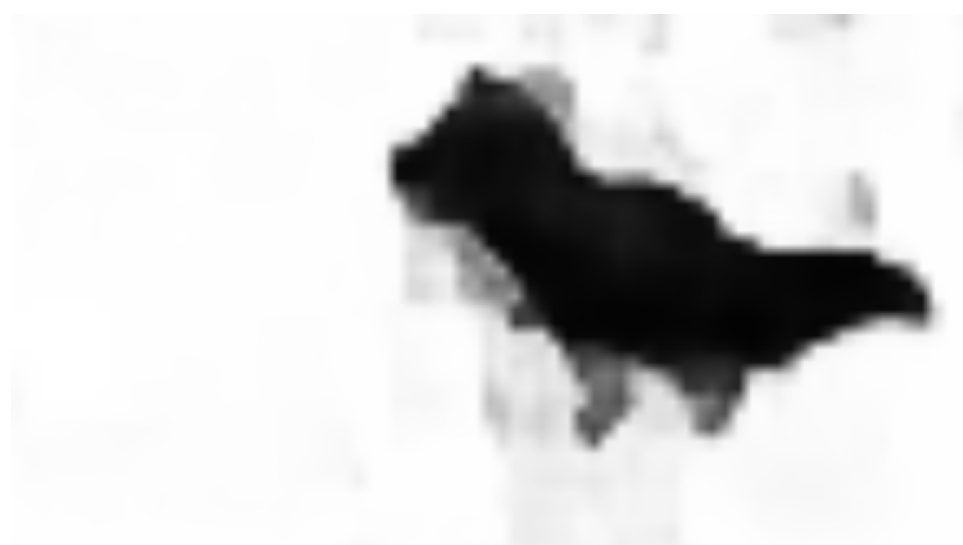

Supplement: Supplementary file 1 [file Motion_VIS.pdf]
